# Supplementary material for: Topics in Mode Conversion Theory and the Group Theoretical Foundations of Path Integrals
Source: arXiv:0901.1650 source file (2009-01-12)
Supplement: Supplementary file 1 [file Appendix.tex]

%%%%%%%%%%%%%%%%%%%%%%%%%%%%%%%%%%%%%%%%%%%%%%%%%%%%%%%%%%%%%%%%%%%%%%%%%%
%
% Ph.D. dissertation manuscript
% Appendicies
%
% Andrew Stephen Richardson (Fall 2007)
% College of William and Mary
% Department of Physics
% Prof. Eugene Tracy, advisor
%
% Based on Paul King and Andrew Norman's template (modified by Wirawan Purwanto)
%
%%%%%%%%%%%%%%%%%%%%%%%%%%%%%%%%%%%%%%%%%%%%%%%%%%%%%%%%%%%%%%%%%%%%%%%%%%

\comment{% husimi inversion and "why HW?"
 
\chapter{Inversion of the Husimi function}

See ``What do phase space methods tell us about disordered quantum systems?'' by Ingold, Wobst, Aulbach, H\"anggi

\[
W(x,k)=\int \frac{\text{d} u \text{d}v}{2\pi}\frac{\text{d}x' \text{d}k'}{2\pi} \exp \left[
\frac{\sigma^2 u^2}{2}+\frac{v^2}{8\sigma^2}+\text{i}(x'-x)u + \text{i}(k'-k)v
\right] \rho(x',k')
\]
where the Husimi function is given by
\[
\rho(x,k)=\frac{1}{\pi} \int \text{d}x' \text{d}k' \exp\left[ -\frac{(x-x')^2}{2\sigma^2}-2\sigma^2(k-k')^2 \right] W(x',k')
\]
and the Wigner function is
\[
W(x,k)=\int dy \; e^{\text{i}ky} \psi^*(x+\frac{y}{2}) \psi(x-\frac{y}{2})
\]

\chapter{Why is the Heisenberg-Weyl Group Important?}

Why is it that the Heisenberg-Weyl group seems to come up so often in problems in physics?  Whether you are doing quantum mechanics, classical wave mechanics or just taking a Fourier transform, the Heisenberg-Weyl group is lurking in the background.  Why does it come up in these and many other fields?  This paper is an attempt to show that the Heisenberg-Weyl group arises when the representations of the translation group are considered.

\section{Representing the Translation Group}

Consider the group of translations in $\mathbb{R}^n$.  This is a commutative group, so its irreducible representations are 1-dim operators in the Hilbert space $\mathcal{H}=L_2(\mathbb{R}^n)$.  Since these operators are an irreducible representation, we have that $T_x T_{x'} = T_{x+x'}, \forall x,x' \in \mathbb{R}^n$.  Also, their eigenvectors must form a complete, orthogonal basis for the space, and the eigenvectors must be phases.  We can therefore write the eigenvalue equation as
\[
T_x \vert \alpha \rangle = e^{i \alpha(x)} \vert \alpha \rangle
\]
where we have labeled the states by the phase of the eigenvalue.  Manipulating this equation, and using the fact that the group is commutative, one arrives at the relation
\[
T_{x'} T_x \vert \alpha \rangle = e^{i \alpha(x)}e^{i \alpha(x')} \vert \alpha \rangle.
\]
This implies that $\alpha$ is a linear function of $x$, or $\alpha(x)+\alpha(x')=\alpha(x+x')$.  We can therefore write $\alpha$ in the standard form $\alpha(x)=k\cdot x= \langle k, x \rangle$ where $k$ is a linear functional from the dual space $(\mathbb{R}^n)^*$.  Taking different choices of $k$ gives us different irreducible representations of the translation group.  We can associate with each $k \in (\mathbb{R}^n)^*$ an irrep $T_x \vert k \rangle = e^{i k\cdot x}\vert k \rangle$.

\section{The Automorphisms of the Translation Group}

Notice that $(\mathbb{R}^n)^*$ has the same structure as $\mathbb{R}^n$, in particular, we can construct the group of shifts on $(\mathbb{R}^n)^*$.  Denote these by $S_k$, and notice that
\[
S_k S_{k'} = S_{k+k'} \qquad \text{and} \qquad S_{k'}\vert k \rangle = \vert k + k' \rangle.
\]
The second equality is simply saying that the $S_k$'s take one irrep of translations in $x$ to another, i.e., the $S_k$'s are group automorphisms of the translation group.  We can now ask about the eigenvectors of the $S_k$ operators.  By similar arguments as used above, we must have that
\[
S_k \vert \beta \rangle = e^{i \beta(k)} \vert \beta \rangle
\]
Again, the phase must be linear in $k$ and $\beta$; choose $\beta(k)=-\beta\cdot k$.

\section{Combining $T_x$ and $S_k$}

We have two sets of operators that can act on the same space, so it is reasonable to ask what their commutator is.  Using the relationships above, we find that 
\[
S_{k}^{-1}T_x^{-1}S_k T_x \vert k' \rangle = e^{-ik\cdot x} \vert k' \rangle, \quad \forall \ k'.
\]
This can also be written as the operator identity
\[
S_{k}^{-1}T_x^{-1}S_k T_x = e^{-ik\cdot x} \text{Id} .
\]

 We would now like to know how the operator $T_x$ acts on the states $\vert \beta \rangle$.  Let's start with the eigenvector equation for $S_k$, and then try the enzatz $T_x \vert \beta \rangle = \vert \beta + x \rangle$, which is what we might expect given how the $S_k$ act on the $T_x$ eigenvectors.
 \begin{eqnarray*}
 S_k \vert \beta \rangle &=& e^{-i\beta \cdot k}\vert \beta \rangle\\
 T_x S_k \vert \beta \rangle &=& e^{-i\beta \cdot k} T_x \vert \beta \rangle\\
 S_k^{-1} T_x S_k \vert \beta \rangle &=& e^{-i\beta \cdot k} S_k^{-1} \vert \beta +x \rangle\\
 T_x^{-1}S_k^{-1} T_x S_k \vert \beta \rangle &=& e^{-i\beta \cdot k} e^{i(\beta +x)\cdot k} \vert \beta \rangle\\
( S_{k}^{-1}T_x^{-1}S_k T_x)^{-1} \vert \beta \rangle &=& e^{ix\cdot k} \vert \beta \rangle
 \end{eqnarray*}
 This gives us the same commutator relation as before, so it show that our enzatz works, and we can label the eigenvectors of $S_k$ with $x$.
 
\section{Bringing it Together to get the Heisenberg-Weyl group}
 
We've shown that, starting with shifts in $\mathbb{R}^n$, we can construct the set of irreducible representations, which has the same structure as $\mathbb{R}^n$.  So there exists a group of shifts in the space of irreps (commonly called momentum space), and this new group of shifts can be labeled by our original space.  Now, instead of identifying $\mathbb{R}^n$ with its dual $\widehat {\mathbb{R}^n}$, we can embed both into a space of larger dimension.  In order to define the operators $T_x$ and $S_k$ on the new space in such a way as preserve their commutator, we will need one more dimension to describe the phase.  We now have a space $\mathbb{R}^{2n+1}$, and a group product law can be defined on the space with the help of the $T_x$, $S_k$ commutator.  The product law is then
\[
(x_1,k_1,\lambda_1) (x_2,k_2,\lambda_2) = (x_1+x_2,k_1+k_2,\lambda_1+\lambda_2+\frac{1}{2}(x_1 k_2-k_1 x_2)).
\]
And there it is; the Heisenberg-Weyl group.

}% end of husimi inversion and "why HW?"
